# Supplementary material for: Adapting Pre-trained Generative Models for Extractive Question Answering
Source: arXiv:2311.02961 source file (2023-11-06)
Supplement: Supplementary file 1 [file appendix.tex]

\section{Appendix}
\label{sec:appendix}
